# Supplementary material for: Kick Back & Relax++: Scaling Beyond Ground-Truth Depth with SlowTV & CribsTV
Source: arXiv:2403.01569 source file (2024-03-03)
Supplement: Supplementary file 2 [file supp_araug.tex]

% Supplementary aspect ratio augmentation visualizations.

% \subfloat[Original (16:9)]{\includegraphics[width=0.345\linewidth]{araug/00_00}}\hfill
% \subfloat[4:5]{\includegraphics[width=.145\linewidth]{araug/00_04}}\hfill
% \subfloat[Original (16:9)]{\includegraphics[width=0.245\linewidth]{araug/01_00}}\hfill
% \subfloat[5:3]{\includegraphics[width=.245\linewidth]{araug/01_01}}
% \\[-0.5ex]
% \subfloat[Original (16:9)]{\includegraphics[width=0.245\linewidth]{araug/05_00}}\hfill
% \subfloat[2:1]{\includegraphics[width=.245\linewidth]{araug/05_05}}\hfill
% \subfloat[Original (16:9)]{\includegraphics[width=0.295\linewidth]{araug/09_00}}\hfill
% \subfloat[1:1]{\includegraphics[width=.195\linewidth]{araug/09_02}}
\vspace{-0.25cm}

\subfloat[Original (16:9)]{\includegraphics[width=0.69\linewidth]{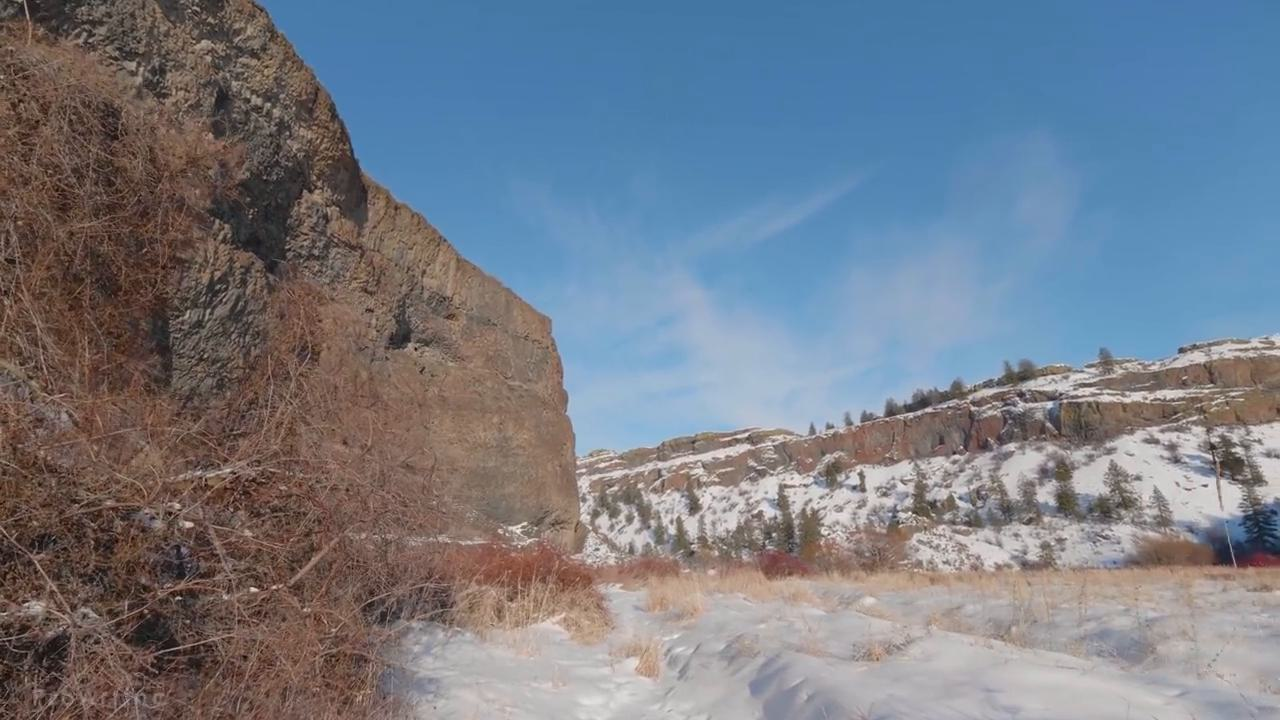}}\hfill
\subfloat[4:5]{\includegraphics[width=.29\linewidth]{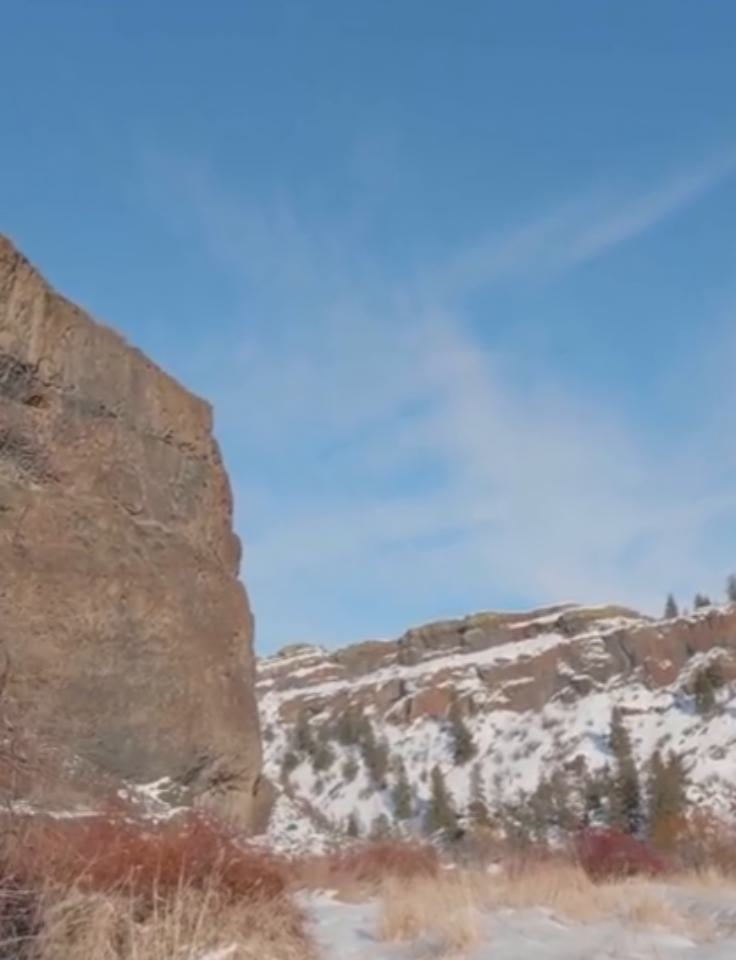}}\hfill
\subfloat[Original (16:9)]{\includegraphics[width=0.49\linewidth]{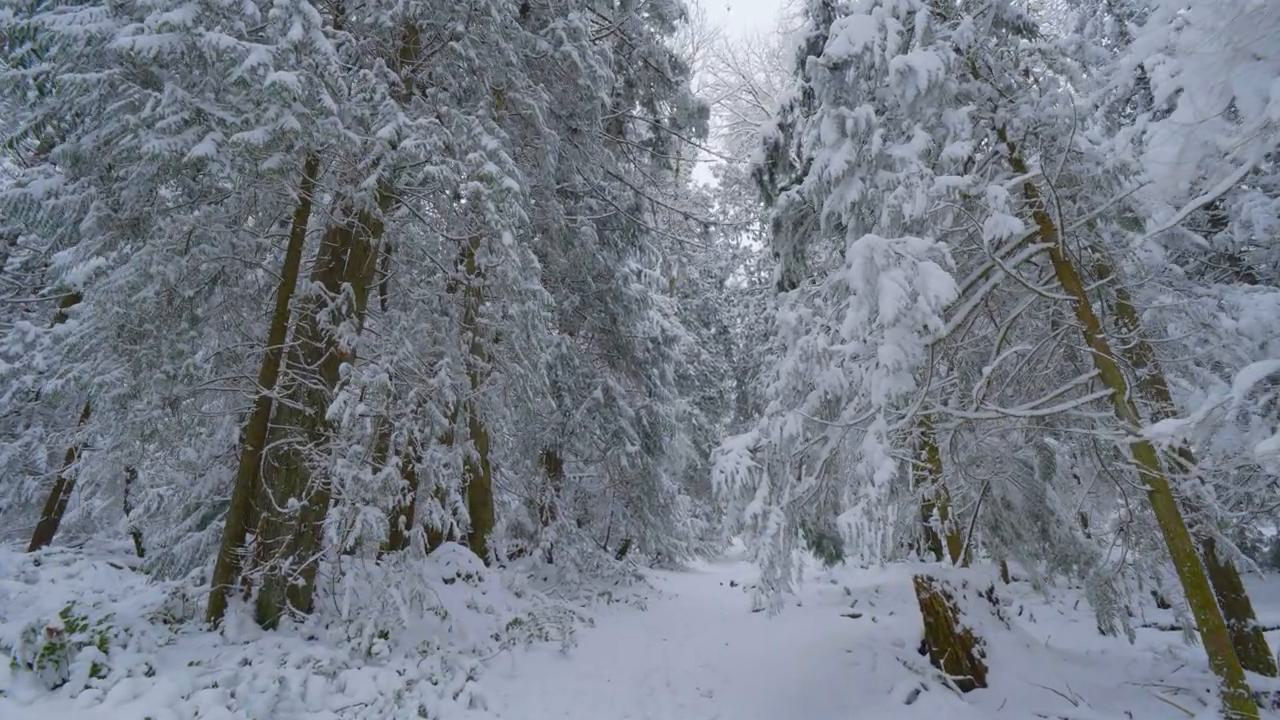}}\hfill
\subfloat[5:3]{\includegraphics[width=.49\linewidth]{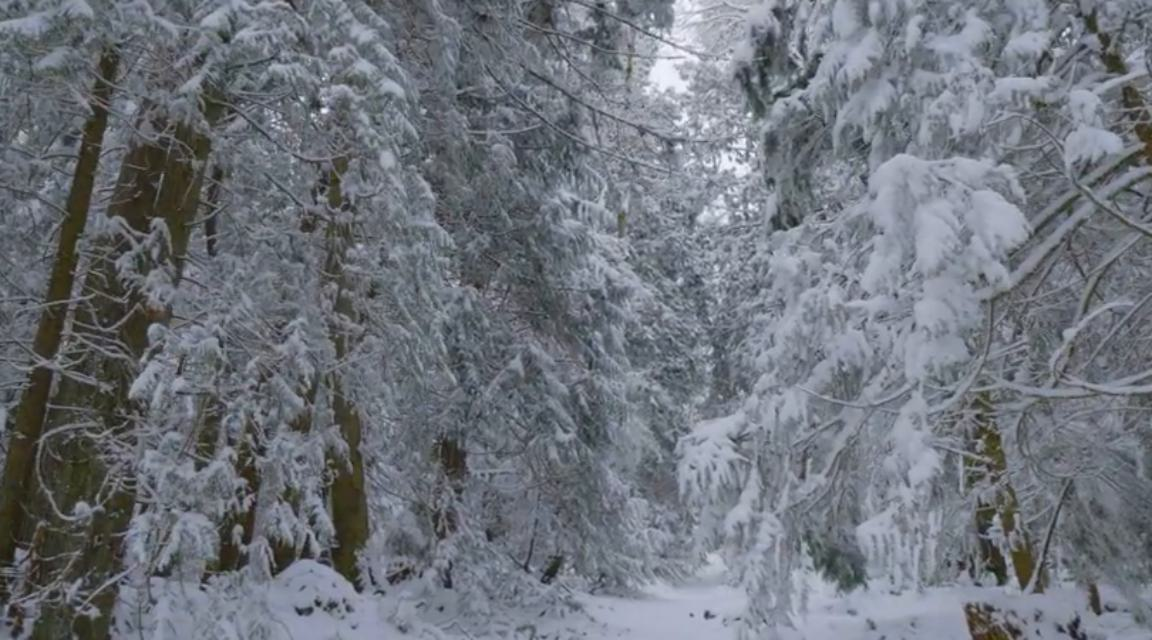}}
\\[-0.5ex]
\subfloat[Original (16:9)]{\includegraphics[width=0.49\linewidth]{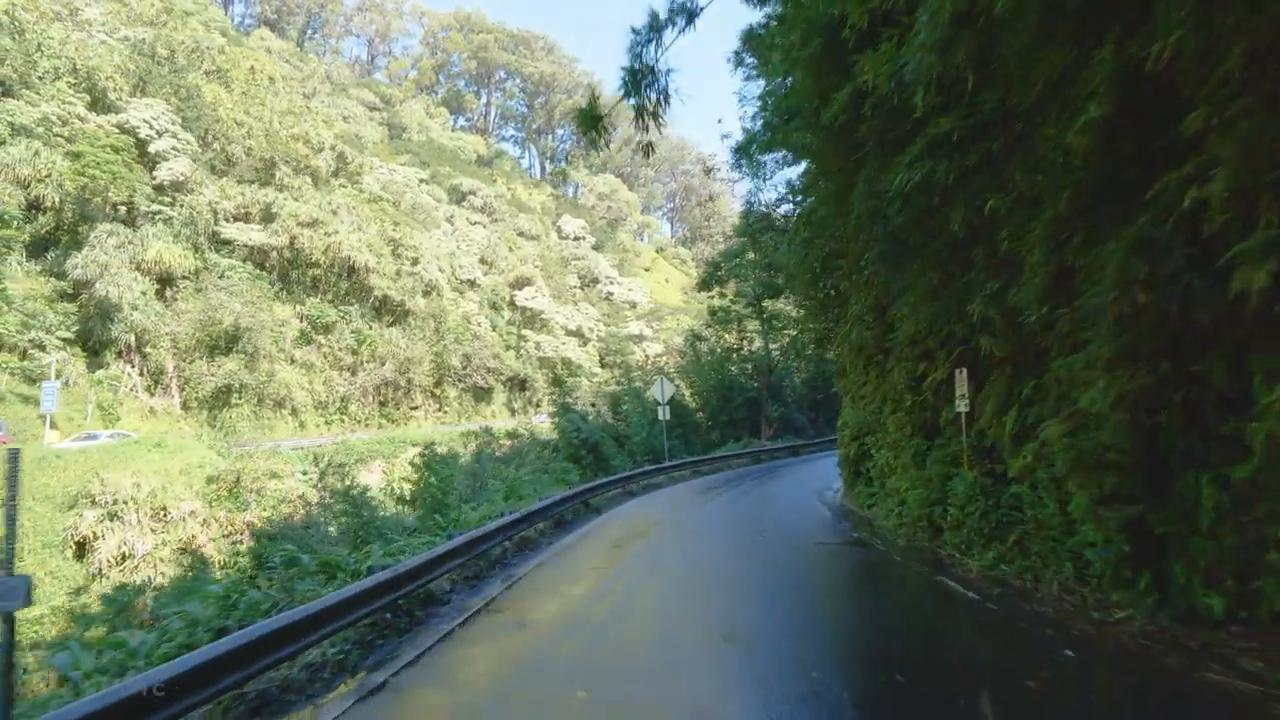}}\hfill
\subfloat[2:1]{\includegraphics[width=.49\linewidth]{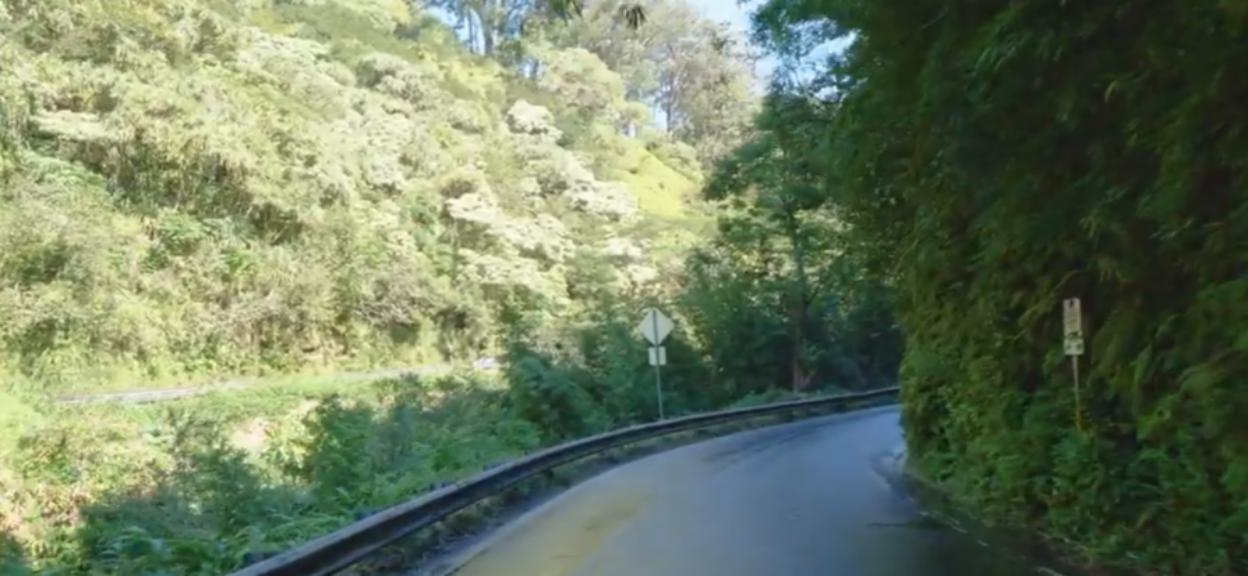}}\hfill
\subfloat[Original (16:9)]{\includegraphics[width=0.59\linewidth]{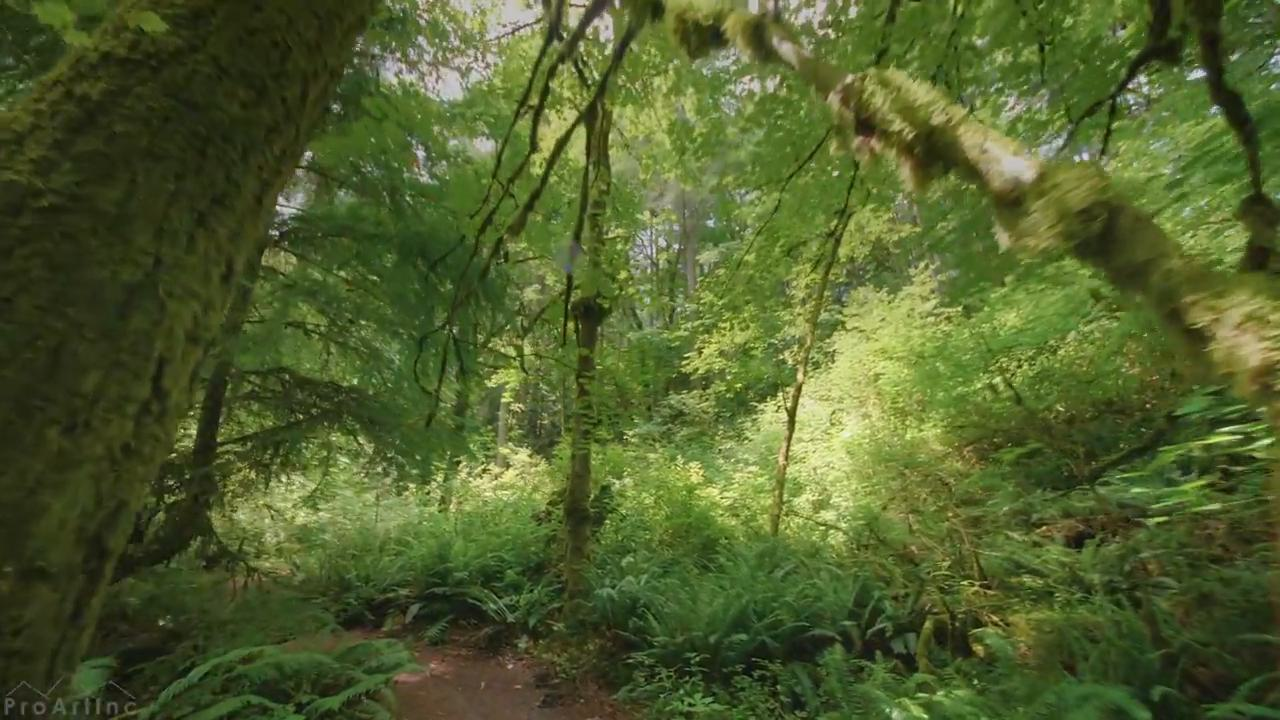}}\hfill
\subfloat[1:1]{\includegraphics[width=.39\linewidth]{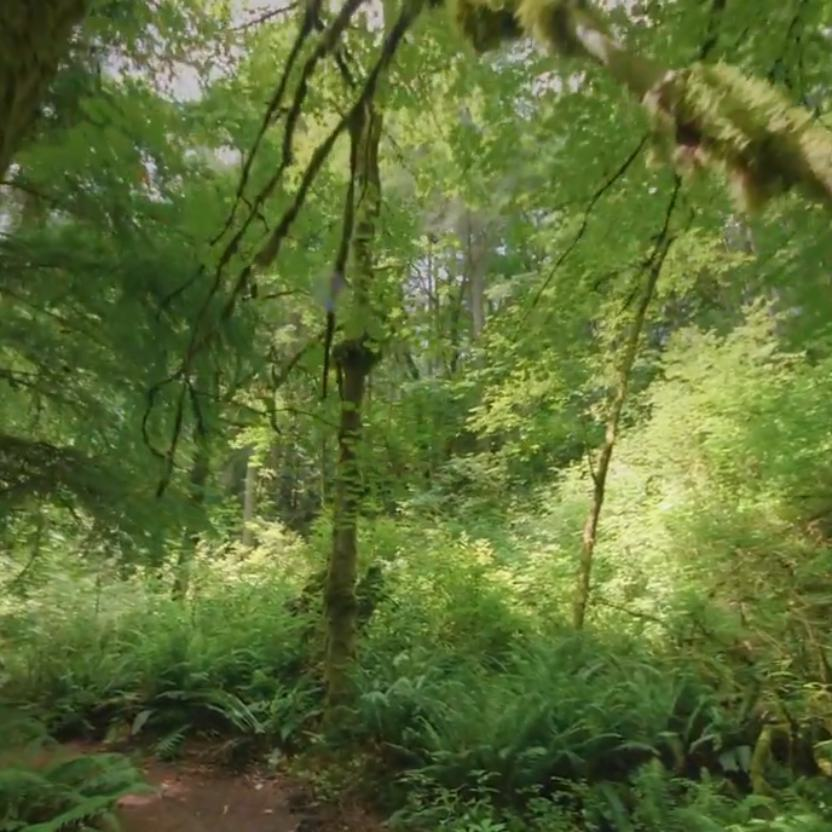}}

\mycaption{\acs{araug}}{%
Additional augmentations used to diversify the variety of image shapes and object scales seen by the network.
}
\vspace{-0.5cm}
