# Supplementary material for: Kick Back & Relax++: Scaling Beyond Ground-Truth Depth with SlowTV & CribsTV
Source: arXiv:2403.01569 source file (2024-03-03)
Supplement: Supplementary file 3 [file supp_slowtv.tex]

% Supplementary SlowTV images (one per video). 

\newcommand{\numrows}{8}
\newcommand{\numcols}{5}
\def\w{.2}

\newcounter{i}
\newcounter{j}
\newcounter{ij}

% Zero-padding for sequence number
\renewcommand{\theij}{%
  \ifnum\value{ij}<10 0\fi
  \ifnum\value{ij}<100 000\fi
  \the\value{ij}%
}

\forloop{i}{0}{\value{i}<\numrows}{%
    \forloop{j}{0}{\value{j}<\numcols}{%
        \setcounter{ij}{\value{i}*\numcols + \value{j}}%
        \includegraphics[width=\w\linewidth]{slowtv_all/\theij}%
    } \\[-0.3ex]

}
\mycaption{\acl{stv} Dataset}{%
We show one frame per video from the proposed \acl{stv}. 
The dataset contains a diverse set of environments in a range of environmental conditions. 
The final dataset has a total of 1.7M images, with 1.15M natural, 400k driving and 180k underwater.
}
