# Supplementary material for: Kick Back & Relax++: Scaling Beyond Ground-Truth Depth with SlowTV & CribsTV
Source: arXiv:2403.01569 source file (2024-03-03)
Supplement: Supplementary file 4 [file supp_slowtv_map.tex]

% Supplementary SlowTV video locations on world map.

\includegraphics[width=0.8\linewidth]{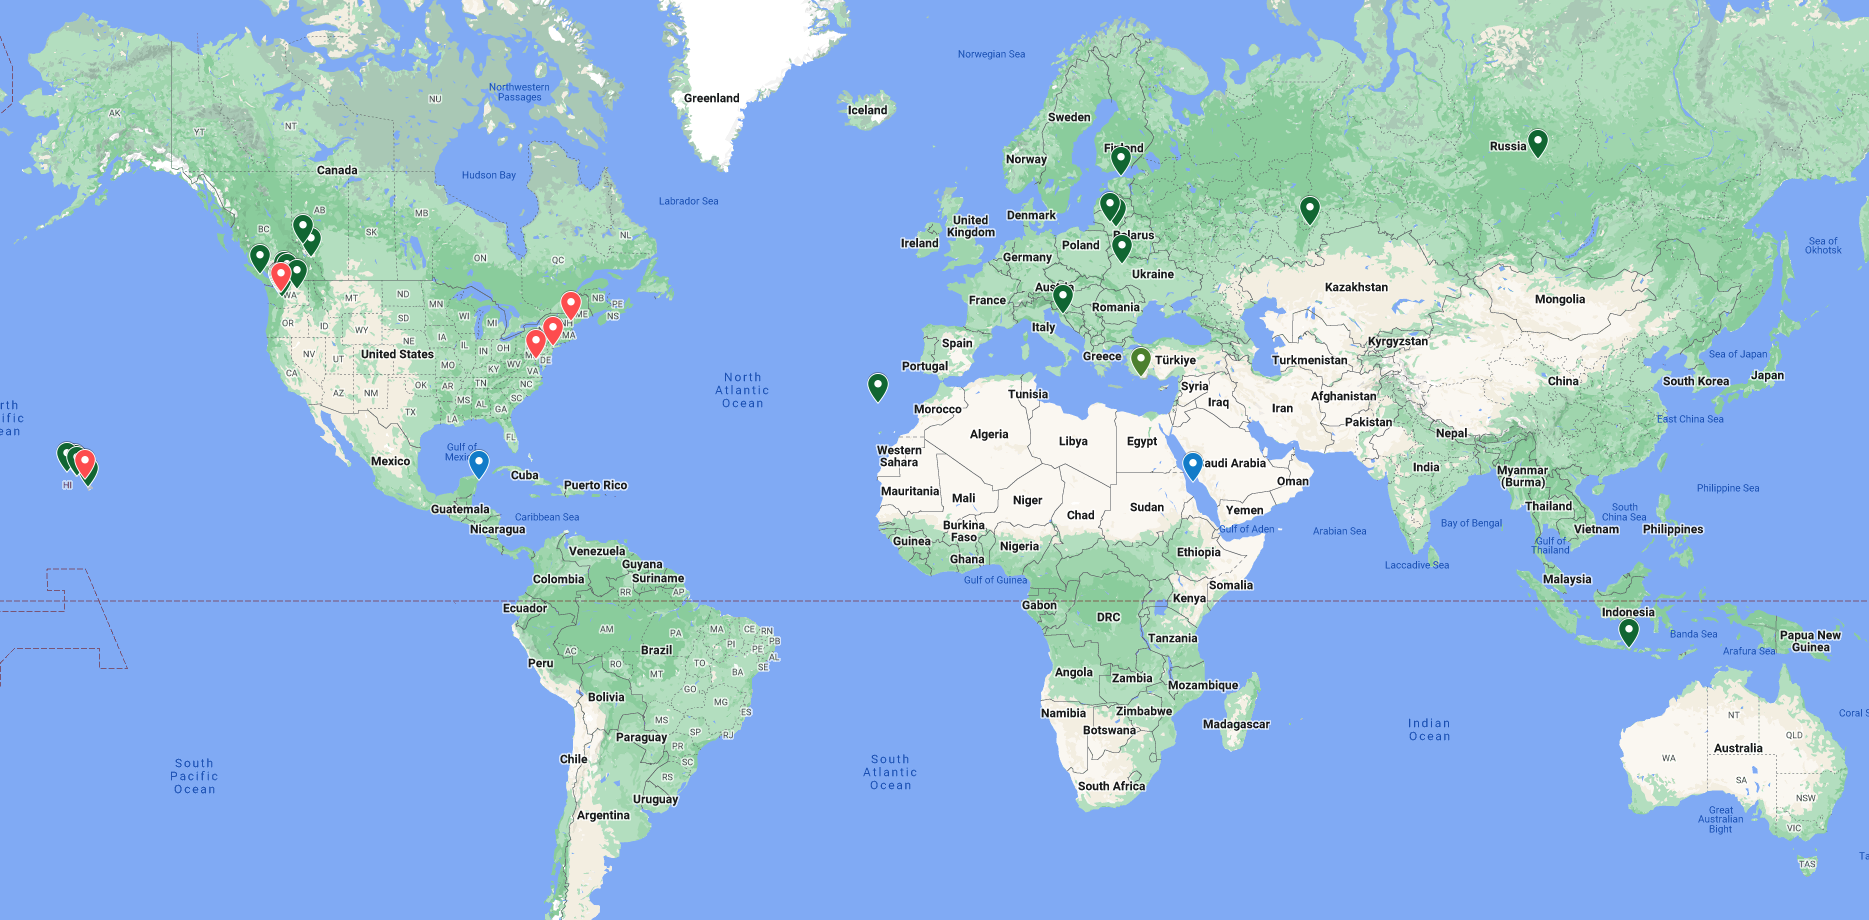}

\mycaption{\acl{stv} Map}{%
We show the map location for each sequence in \acl{stv}.
The distribution of locations ensures that the training data is highly diverse.
\textcolor{ForestGreen}{\textbf{Green}}=Natural, \textcolor{red}{\textbf{Red}}=Driving, \textcolor{blue}{\textbf{Blue}}=Underwater.
}
