# Supplementary material for: Kick Back & Relax++: Scaling Beyond Ground-Truth Depth with SlowTV & CribsTV
Source: arXiv:2403.01569 source file (2024-03-03)
Supplement: Supplementary file 5 [file supp_learnk.tex]

% \footnotesize

\mycaption{Learning Camera Intrinsics}{%
Performance when training on a single dataset (Kitti or \acl{mc}) and learning camera intrinsics. 
If the cameras are not perfectly calibrated, learning the intrinsics can improve accuracy. 
}

\begin{tabular}{@{}lllllll@{}}
\toprule
              &    \multicolumn{3}{c}{\textbf{\acl{kez}}} \\ 
              \cmidrule(lr){2-4}  
              &     Rel\down &          F\up & $\delta_{.25}$\up    \\ 
\midrule
     Baseline  & \nbest{5.69} &  \best{60.88} &     \nbest{95.89}  \\ 
Learn \acs{Cam} &  \best{5.68} & \nbest{60.81} &      \best{95.90} \\ 
\bottomrule
\end{tabular}
\quad
\begin{tabular}{@{}lllllll@{}}
\toprule
              &     \multicolumn{3}{c}{\textbf{\acs{mc}}} \\ 
              \cmidrule(lr){2-4}  
                &      Rel\down &          F\up & $\delta_{.25}$\up \\ 
\midrule
     Baseline   & \nbest{16.66} & \nbest{14.20} &     \nbest{77.18} \\ 
Learn \acs{Cam} &  \best{16.12} &  \best{14.77} &      \best{78.40} \\ 
\bottomrule
\end{tabular}
