# Supplementary material for: Kick Back & Relax++: Scaling Beyond Ground-Truth Depth with SlowTV & CribsTV
Source: arXiv:2403.01569 source file (2024-03-03)
Supplement: Supplementary file 6 [file supp_motion.tex]

\scriptsize
\addtolength{\tabcolsep}{0.05em}
\def\mc{\multicolumn}

\mycaption{Monodepth2~\cite{Godard2019} Losses}{%
The minimum reconstruction loss and automasking from Monodepth2 serve as valuable proxies to increase robustness to dynamic objects, while remaining simple and efficient. 
}

\begin{tabular}{@{}lllllllllllllllllllll@{}}
\toprule
                             & \mc{2}{c}{\textbf{Multi-task}} & \mc{2}{c}{\bf\acs{keb}}            & \mc{2}{c}{\bf\acs{mc}}             & \mc{2}{c}{\bf\acs{ddad}}      & \mc{2}{c}{\bf\acs{dio}}       & \mc{2}{c}{\bf\acs{sintel}}    & \mc{2}{c}{\bf\acs{syns}}      & \mc{2}{c}{\bf\acs{dii}}       & \mc{2}{c}{\bf\acl{nyud}}          & \mc{2}{c}{\bf\acs{tum}}       \\  
                                       \cmidrule(lr){2-3}                   \cmidrule(lr){4-5}                   \cmidrule(lr){6-7}              \cmidrule(lr){8-9}             \cmidrule(lr){10-11}            \cmidrule(lr){12-13}            \cmidrule(lr){14-15}            \cmidrule(lr){16-17}                \cmidrule(lr){18-19}  \cmidrule(lr){20-21}
                             &   \acs{rank}\down &        \acs{relimp}\up &        Rel\down &             F\up &         Rel\down &            F\up &      Rel\down &          F\up &      Rel\down &  \acs{d25}\up &      Rel\down &          F\up &      Rel\down &          F\up &      Rel\down &  \acs{d25}\up &       Rel\down &     \acs{d25}\up &      Rel\down &  \acs{d25}\up \\
\midrule
         Baseline & \nbest{1.89} & \nbest{0.00} & \nbest{9.00} & \nbest{53.50} &  \best{16.89} &  \best{14.66} & \nbest{23.57} & \nbest{11.13} & \nbest{35.99} &     \nbest{52.70} & \nbest{35.33} & \nbest{38.15} & \nbest{25.47} & \nbest{15.73} & \nbest{17.91} &     \nbest{75.03} & \nbest{21.68} &     \nbest{71.41} & \nbest{17.69} &     \nbest{75.67} \\ 
MinRec+Automask &  \best{1.11} &  \best{7.01} &  \best{6.50} &  \best{55.62} & \nbest{16.96} & \nbest{14.48} &  \best{18.49} &  \best{11.64} &  \best{35.62} &      \best{52.95} &  \best{34.97} &  \best{38.83} &  \best{24.44} &  \best{16.25} &  \best{16.85} &      \best{76.50} &  \best{14.27} &      \best{80.54} &  \best{17.23} &      \best{76.23} \\ 
\bottomrule
\end{tabular}
